# Supplementary material for: Towards a Game-Theoretic Security Analysis of Off-Chain Protocols
Source: arXiv:2109.07429 source file (2022-10-24)
Supplement: Supplementary file 1 [file appendix.tex]

\input{includes/appendices/secproofs.tex}
\input{includes/CSFappendix.tex}
