# Supplementary material for: Towards a Game-Theoretic Security Analysis of Off-Chain Protocols
Source: arXiv:2109.07429 source file (2022-10-24)
Supplement: Supplementary file 2 [file subgames.tex]

\subsection{Subgames of the Closing Game} \label{app:subgames}
In the following all the subgames needed for the closing game $G_c(A)$ are defined.

The subgames $S_1$ and $S_2$ in \Cref{tbl:S1} and \Cref{tbl:S2} cover the case where a channel update is proposed by $A$, although $A$ has already signed an honest collaborative closing attempt. In $S_1$ the update is from channel state $(a,b)$ to $(a+p_A,b-p_A)$, whereas in $S_2$ the suggested update is $(a-p_B, b+p_B)$.

\begin{figure}
	\centering
	\begin{tikzpicture}[->,>=stealth',auto,node distance=2cm, el/.style = {inner sep=2pt, align=left, sloped}]
		\node (1) at (1.75,0.75) {\color{olive}$B$};
		
		%B block top
		\node (20) at (1,-2.25) {\color{teal} $A$};
		\node (2) at (1.75,-2.75) {\color{teal}$A$} ; 
		\node (3) at (-1.,-0.25) {\color{teal}$A$};
		\node (21) at (-1,0.5) {$(\alpha,\alpha-\epsilon)$};
		\node (24) at (-0.15,-1.25) {$(\alpha,\alpha)$};
		
		%A block middle
		\node (22) at (-2.,-3.25) {$(b-f+\alpha,-b)$};
		\node (23) at (-3.5,-2.75) {$(-d_B+\alpha,d_B+\alpha-\epsilon)$};
				
		%A block left
		\node (8) at (-3.25,-2) {$(-a,-b)$};
		\node (9) at (-1.75,-2.) {$(\alpha-\epsilon,\alpha)$};
		\node (10) at (-2.25,-0.5) {\color{olive}$B$};
		
		%A block right
		\node (5) at (1.75,-5.75) {\color{olive}$B$};
		\node (6) at (-1,-4) {$(\rho+\alpha-\epsilon,\rho+\alpha)$};
		\node (7) at (1,-4.25) {\color{olive}$B$};
		
		%B block middle
		\node (11) at (-1.25,-5.5) {$(-a{\color{red}-p_A}+\rho,a{\color{red}+p_A}-f+\rho+\alpha)$};
		\node (12) at (-3.25,-5) {$(d_A+\rho+\alpha-\epsilon,-d_A+\rho+\alpha)$};
		
		%B block left
		\node (13) at (-5,-0.75) {$(-a,a-f+\alpha)$};
		\node (14) at (-4.35,-1.25) {$(d_A+\alpha-\epsilon,-d_A+\alpha)$};
		
		%B block right
		\node (15) at (1.75,-8.25) {\color{teal}$A$};
		\node (16) at (-0.5,-8) {$(\rho+\alpha,\rho+\alpha-\epsilon)$};
		\node (17) at (-2.5,-7.5) {$(-a{\color{red}-p_A}+\rho,-b{\color{red}+p_A}+\rho)$};
		\node (4) at (-3.75,-6.75) {$({\color{red}-p_A}+\rho+\alpha,{\color{red}p_A}+\rho+\alpha)$};
		
		%A block bottom
		\node (18) at (-3,-9) {$(b{\color{red}-p_A}-f+\rho+\alpha,-b{\color{red}+p_A}+\rho)$};
		\node (19) at (-0.5,-9.5) {$(-d_B+\rho+\alpha,d_B+\rho+\alpha-\epsilon)$};
		
		{\color{olive}
		\path (1) edge node [left, pos=0.5] {\tiny $A$}  (2);
		\path (1) edge node [above, pos=0.5] {\tiny $I$}  (3); 
		\path (1) edge node [left]  {\tiny $D$} (20);
		\path (1) edge node [above]  {\tiny $H$} (21);
		\path (1) edge node [left] {\tiny $S$} (24); }
		
		{\color{teal}
		\path (2) edge node [left, pos=0.3] {\tiny $I$}  (5);
		\path (2) edge node [above] {\tiny $H$}  (6);
		\path (2) edge node [left] {\tiny $D$}  (7);
		\path (3) edge node [above, pos=0.5] {\tiny $I$}  (8);

		\path (3) edge node [left] {\tiny $H$}  (9);
		\path (3) edge node [above] {\tiny $D$}  (10); 
		
		\path (20) edge node [below] {\tiny $I$} (23); 
		\path (20) edge node [below] {\tiny $P$} (22);}
		
		{\color{olive}
		\path (7) edge node [below] {\tiny $P$}  (11); 
		\path (7) edge node [below] {\tiny $I$}  (12);
		
		\path (10) edge node [above, pos=0.7] {\tiny $P$}  (13);
		\path (10) edge node [below] {\tiny $I$}  (14);
		
		\path (5) edge node [left] {\tiny $D$}  (15);
		\path (5) edge node [above] {\tiny $H$}  (16); 
		\path (5) edge node [above] {\tiny $I$}  (17);
		\path (5) edge node [above] {\tiny $S$}  (4);}
		
		{\color{teal}
		\path (15) edge node [below] {\tiny $P$}  (18);
		\path (15) edge node [below] {\tiny $I$}  (19);}
	\end{tikzpicture}
	\caption{Subgame $S_{1}$ with Update $(a,b)\mapsto (a+p_A,b-p_A)$.}
	\label{tbl:S1}
\end{figure}

\begin{figure}
	\centering
	\begin{tikzpicture}[->,>=stealth',auto,node distance=2cm, el/.style = {inner sep=2pt, align=left, sloped}]
		\node (1) at (1.75,0.75) {\color{olive}$B$};
		
		%B block top
		\node (20) at (1,-2.25) {\color{teal} $A$};
		\node (2) at (1.75,-2.75) {\color{teal}$A$} ; 
		\node (3) at (-1.,-0.25) {\color{teal}$A$};
		\node (21) at (-1,0.5) {$(\alpha,\alpha-\epsilon)$};
		\node (24) at (-0.15,-1.25) {$(\alpha,\alpha)$};
		
		%A block middle
		\node (22) at (-2.,-3.25) {$(b-f+\alpha,-b)$};
		\node (23) at (-3.5,-2.75) {$(-d_B+\alpha,d_B+\alpha-\epsilon)$};
				
		%A block left
		\node (8) at (-3.25,-2) {$(-a,-b)$};
		\node (9) at (-1.75,-2.) {$(\alpha-\epsilon,\alpha)$};
		\node (10) at (-2.25,-0.5) {\color{olive}$B$};
		
		%A block right
		\node (5) at (1.75,-5.75) {\color{olive}$B$};
		\node (6) at (-1,-4) {$(\rho+\alpha-\epsilon,\rho+\alpha)$};
		\node (7) at (1,-4.25) {\color{olive}$B$};
		
		%B block middle
		\node (11) at (-1.25,-5.5) {$(-a{\color{red}+p_B}+\rho,a{\color{red}-p_B}-f+\rho+\alpha)$};
		\node (12) at (-3.25,-5) {$(d_A+\rho+\alpha-\epsilon,-d_A+\rho+\alpha)$};
		
		%B block left
		\node (13) at (-5,-0.75) {$(-a,a-f+\alpha)$};
		\node (14) at (-4.35,-1.25) {$(d_A+\alpha-\epsilon,-d_A+\alpha)$};
		
		%B block right
		\node (15) at (1.75,-8.25) {\color{teal}$A$};
		\node (16) at (-0.5,-8) {$(\rho+\alpha,\rho+\alpha-\epsilon)$};
		\node (17) at (-2.5,-7.5) {$(-a{\color{red}+p_B}+\rho,-b{\color{red}-p_B}+\rho)$};
		\node (4) at (-3.75,-6.75) {$({\color{red}p_B}+\rho+\alpha,{\color{red}-p_B}+\rho+\alpha)$};
		
		%A block bottom
		\node (18) at (-3,-9) {$(b{\color{red}+p_B}-f+\rho+\alpha,-b{\color{red}-p_B}+\rho)$};
		\node (19) at (-0.5,-9.5) {$(-d_B+\rho+\alpha,d_B+\rho+\alpha-\epsilon)$};
		
		{\color{olive}
		\path (1) edge node [left, pos=0.5] {\tiny $A$}  (2);
		\path (1) edge node [above, pos=0.5] {\tiny $I$}  (3); 
		\path (1) edge node [left]  {\tiny $D$} (20);
		\path (1) edge node [above]  {\tiny $H$} (21);
		\path (1) edge node [left] {\tiny $S$} (24); }
		
		{\color{teal}
		\path (2) edge node [left, pos=0.3] {\tiny $I$}  (5);
		\path (2) edge node [above] {\tiny $H$}  (6);
		\path (2) edge node [left] {\tiny $D$}  (7);
		\path (3) edge node [above, pos=0.5] {\tiny $I$}  (8);

		\path (3) edge node [left] {\tiny $H$}  (9);
		\path (3) edge node [above] {\tiny $D$}  (10); 
		
		\path (20) edge node [below] {\tiny $I$} (23); 
		\path (20) edge node [below] {\tiny $P$} (22);}
		
		{\color{olive}
		\path (7) edge node [below] {\tiny $P$}  (11); 
		\path (7) edge node [below] {\tiny $I$}  (12);
		
		\path (10) edge node [above, pos=0.7] {\tiny $P$}  (13);
		\path (10) edge node [below] {\tiny $I$}  (14);
		
		\path (5) edge node [left] {\tiny $D$}  (15);
		\path (5) edge node [above] {\tiny $H$}  (16); 
		\path (5) edge node [above] {\tiny $I$}  (17);
		\path (5) edge node [above] {\tiny $S$}  (4);}
		
		{\color{teal}
		\path (15) edge node [below] {\tiny $P$}  (18);
		\path (15) edge node [below] {\tiny $I$}  (19);}
	\end{tikzpicture}
	\caption{Subgame $S_{2}$ with Update $(a,b)\mapsto (a-p_B,b+p_B)$.}
	\label{tbl:S2}
\end{figure}

The subgames $S_1'$ and $S_2'$ in \Cref{tbl:S1p} and \Cref{tbl:S2p} are very similar to $S_1$ and $S_2$. They only differ in the fact, that the existing partially signed collaborative closing attempt was dishonest. That means, $A$ proposed an unfair split, increasing her outcome by value $c>0$.

\begin{figure}
	\centering
	\begin{tikzpicture}[->,>=stealth',auto,node distance=2cm, el/.style = {inner sep=2pt, align=left, sloped}]
		\node (1) at (1.75,0.75) {\color{olive}$B$};
		
		%B block top
		\node (20) at (1,-2.25) {\color{teal} $A$};
		\node (2) at (1.75,-2.75) {\color{teal}$A$} ; 
		\node (3) at (-1.,-0.25) {\color{teal}$A$};
		\node (21) at (-1,0.5) {$(\alpha,\alpha-\epsilon)$};
		\node (24) at (-0.15,-1.25) {$({\color{red}c}+\alpha,{\color{red}-c}+\alpha)$};
		
		%A block middle
		\node (22) at (-2.,-3.25) {$(b-f+\alpha,-b)$};
		\node (23) at (-3.5,-2.75) {$(-d_B+\alpha,d_B+\alpha-\epsilon)$};
				
		%A block left
		\node (8) at (-3.25,-2) {$(-a,-b)$};
		\node (9) at (-1.75,-2.) {$(\alpha-\epsilon,\alpha)$};
		\node (10) at (-2.25,-0.5) {\color{olive}$B$};
		
		%A block right
		\node (5) at (1.75,-5.75) {\color{olive}$B$};
		\node (6) at (-1,-4) {$(\rho+\alpha-\epsilon,\rho+\alpha)$};
		\node (7) at (1,-4.25) {\color{olive}$B$};
		
		%B block middle
		\node (11) at (-1.25,-5.5) {$(-a{\color{red}-p_A}+\rho,a{\color{red}+p_A}-f+\rho+\alpha)$};
		\node (12) at (-3.25,-5) {$(d_A+\rho+\alpha-\epsilon,-d_A+\rho+\alpha)$};
		
		%B block left
		\node (13) at (-5,-0.75) {$(-a,a-f+\alpha)$};
		\node (14) at (-4.35,-1.25) {$(d_A+\alpha-\epsilon,-d_A+\alpha)$};
		
		%B block right
		\node (15) at (1.75,-8.25) {\color{teal}$A$};
		\node (16) at (-0.5,-8) {$(\rho+\alpha,\rho+\alpha-\epsilon)$};
		\node (17) at (-2.5,-7.5) {$(-a{\color{red}-p_A}+\rho,-b{\color{red}+p_A}+\rho)$};
		\node (4) at (-3.75,-6.75) {$({\color{red}c-p_A}+\rho+\alpha,{\color{red}-c+p_A}+\rho+\alpha)$};
		
		%A block bottom
		\node (18) at (-3,-9) {$(b{\color{red}-p_A}-f+\rho+\alpha,-b{\color{red}+p_A}+\rho)$};
		\node (19) at (-0.5,-9.5) {$(-d_B+\rho+\alpha,d_B+\rho+\alpha-\epsilon)$};
		
		{\color{olive}
		\path (1) edge node [left, pos=0.5] {\tiny $A$}  (2);
		\path (1) edge node [above, pos=0.5] {\tiny $I$}  (3); 
		\path (1) edge node [left]  {\tiny $D$} (20);
		\path (1) edge node [above]  {\tiny $H$} (21);
		\path (1) edge node [left] {\tiny $S$} (24); }
		
		{\color{teal}
		\path (2) edge node [left, pos=0.3] {\tiny $I$}  (5);
		\path (2) edge node [above] {\tiny $H$}  (6);
		\path (2) edge node [left] {\tiny $D$}  (7);
		\path (3) edge node [above, pos=0.5] {\tiny $I$}  (8);

		\path (3) edge node [left] {\tiny $H$}  (9);
		\path (3) edge node [above] {\tiny $D$}  (10); 
		
		\path (20) edge node [below] {\tiny $I$} (23); 
		\path (20) edge node [below] {\tiny $P$} (22);}
		
		{\color{olive}
		\path (7) edge node [below] {\tiny $P$}  (11); 
		\path (7) edge node [below] {\tiny $I$}  (12);
		
		\path (10) edge node [above, pos=0.7] {\tiny $P$}  (13);
		\path (10) edge node [below] {\tiny $I$}  (14);
		
		\path (5) edge node [left] {\tiny $D$}  (15);
		\path (5) edge node [above] {\tiny $H$}  (16); 
		\path (5) edge node [above] {\tiny $I$}  (17);
		\path (5) edge node [above] {\tiny $S$}  (4);}
		
		{\color{teal}
		\path (15) edge node [below] {\tiny $P$}  (18);
		\path (15) edge node [below] {\tiny $I$}  (19);}
	\end{tikzpicture}
	\caption{Subgame $S'_{1}$ with Update $(a,b)\mapsto (a+p_A,b-p_A)$.}
	\label{tbl:S1p}
\end{figure}

\begin{figure}
	\centering
	\begin{tikzpicture}[->,>=stealth',auto,node distance=2cm, el/.style = {inner sep=2pt, align=left, sloped}]
		\node (1) at (1.75,0.75) {\color{olive}$B$};
		
		%B block top
		\node (20) at (1,-2.25) {\color{teal} $A$};
		\node (2) at (1.75,-2.75) {\color{teal}$A$} ; 
		\node (3) at (-1.,-0.25) {\color{teal}$A$};
		\node (21) at (-1,0.5) {$(\alpha,\alpha-\epsilon)$};
		\node (24) at (-0.15,-1.25) {$({\color{red}c}+\alpha,{\color{red}-c}+\alpha)$};
		
		%A block middle
		\node (22) at (-2.,-3.25) {$(b-f+\alpha,-b)$};
		\node (23) at (-3.5,-2.75) {$(-d_B+\alpha,d_B+\alpha-\epsilon)$};
				
		%A block left
		\node (8) at (-3.25,-2) {$(-a,-b)$};
		\node (9) at (-1.75,-2.) {$(\alpha-\epsilon,\alpha)$};
		\node (10) at (-2.25,-0.5) {\color{olive}$B$};
		
		%A block right
		\node (5) at (1.75,-5.75) {\color{olive}$B$};
		\node (6) at (-1,-4) {$(\rho+\alpha-\epsilon,\rho+\alpha)$};
		\node (7) at (1,-4.25) {\color{olive}$B$};
		
		%B block middle
		\node (11) at (-1.25,-5.5) {$(-a{\color{red}+p_B}+\rho,a{\color{red}-p_B}-f+\rho+\alpha)$};
		\node (12) at (-3.25,-5) {$(d_A+\rho+\alpha-\epsilon,-d_A+\rho+\alpha)$};
		
		%B block left
		\node (13) at (-5,-0.75) {$(-a,a-f+\alpha)$};
		\node (14) at (-4.35,-1.25) {$(d_A+\alpha-\epsilon,-d_A+\alpha)$};
		
		%B block right
		\node (15) at (1.75,-8.25) {\color{teal}$A$};
		\node (16) at (-0.5,-8) {$(\rho+\alpha,\rho+\alpha-\epsilon)$};
		\node (17) at (-2.5,-7.5) {$(-a{\color{red}+p_B}+\rho,-b{\color{red}-p_B}+\rho)$};
		\node (4) at (-3.75,-6.75) {$({\color{red}c+p_B}+\rho+\alpha,{\color{red}-c-p_B}+\rho+\alpha)$};
		
		%A block bottom
		\node (18) at (-3,-9) {$(b{\color{red}+p_B}-f+\rho+\alpha,-b{\color{red}-p_B}+\rho)$};
		\node (19) at (-0.5,-9.5) {$(-d_B+\rho+\alpha,d_B+\rho+\alpha-\epsilon)$};
		
		{\color{olive}
		\path (1) edge node [left, pos=0.5] {\tiny $A$}  (2);
		\path (1) edge node [above, pos=0.5] {\tiny $I$}  (3); 
		\path (1) edge node [left]  {\tiny $D$} (20);
		\path (1) edge node [above]  {\tiny $H$} (21);
		\path (1) edge node [left] {\tiny $S$} (24); }
		
		{\color{teal}
		\path (2) edge node [left, pos=0.3] {\tiny $I$}  (5);
		\path (2) edge node [above] {\tiny $H$}  (6);
		\path (2) edge node [left] {\tiny $D$}  (7);
		\path (3) edge node [above, pos=0.5] {\tiny $I$}  (8);

		\path (3) edge node [left] {\tiny $H$}  (9);
		\path (3) edge node [above] {\tiny $D$}  (10); 
		
		\path (20) edge node [below] {\tiny $I$} (23); 
		\path (20) edge node [below] {\tiny $P$} (22);}
		
		{\color{olive}
		\path (7) edge node [below] {\tiny $P$}  (11); 
		\path (7) edge node [below] {\tiny $I$}  (12);
		
		\path (10) edge node [above, pos=0.7] {\tiny $P$}  (13);
		\path (10) edge node [below] {\tiny $I$}  (14);
		
		\path (5) edge node [left] {\tiny $D$}  (15);
		\path (5) edge node [above] {\tiny $H$}  (16); 
		\path (5) edge node [above] {\tiny $I$}  (17);
		\path (5) edge node [above] {\tiny $S$}  (4);}
		
		{\color{teal}
		\path (15) edge node [below] {\tiny $P$}  (18);
		\path (15) edge node [below] {\tiny $I$}  (19);}
	\end{tikzpicture}
	\caption{Subgame $S'_{2}$ with  Update $(a,b)\mapsto (a-p_B,b+p_B)$.}
	\label{tbl:S2p}
\end{figure}

The next couple of subgames $S_3$ (\Cref{tbl:S3}), $S_4$ (\Cref{tbl:S4}) represent channel updates that were proposed by $B$, after $A$ tried to close the channel honestly and collaboratively. Similar to before, $S_3$ represents the case where $A$'s balance is increased, therefore an update from $(a,b)$  to $(a+p_A,b-p_A)$. The other subgame $S_4$ handles the case where the update increases $B$'s balance to a new state $(a-p_B,b+p_B)$.

\begin{figure}
	\centering
	\begin{tikzpicture}[->,>=stealth',auto,node distance=2cm, el/.style = {inner sep=2pt, align=left, sloped}]
		\node (1) at (1.75,0.75) {\color{teal}$A$};
		
		%A block top
		\node (20) at (1,-2.25) {\color{olive} $B$};
		\node (2) at (1.75,-3.25) {\color{olive}$B$} ; 
		\node (3) at (-1.,-0.25) {\color{olive}$B$};
		\node (21) at (-1,0.5) {$(\alpha-\epsilon,\alpha)$};
		
		%B block left
		\node (22) at (-2.,-3.25) {$(-a,a-f+\alpha)$};
		\node (23) at (-3.5,-2.75) {$(d_A+\alpha-\epsilon,-d_A+\alpha)$};
				
		%B block middle
		\node (8) at (-2.5,-2) {$(-a,-b)$};
		\node (24) at (-0.,-1.25) {$(\alpha,\alpha)$};
		\node (9) at (-1.,-2.) {$(\alpha,\alpha-\epsilon)$};
		\node (10) at (-2.25,-0.5) {\color{teal}$A$};
		
		%B block right
		\node (4) at (-2.5,-4) {$({\color{red}-p_A}+\rho+\alpha,{\color{red}p_A}+\rho+\alpha)$};
		\node (5) at (1.75,-6.75) {\color{teal}$A$};
		\node (6) at (-1,-4.5) {$(\rho+\alpha,\rho+\alpha-\epsilon)$};
		\node (7) at (1,-5.) {\color{teal}$A$};

		%A block middle
		\node (11) at (-0.75,-6.25) {$(b{\color{red}-p_A}-f+\rho+\alpha,-b{\color{red}+p_A}+\rho)$};
		\node (12) at (-2.75,-5.75) {$(-d_B+\rho+\alpha,d_B+\rho+\alpha-\epsilon)$};
		
		%A block left
		\node (13) at (-5,-0.75) {$(b-f+\alpha,-b)$};
		\node (14) at (-4.25,-1.25) {$(-d_B+\alpha,d_B+\alpha-\epsilon)$};

		%A block right
		\node (15) at (1.75,-8.25) {\color{olive}$B$};
		\node (16) at (-0.5,-8) {$(\rho+\alpha-\epsilon,\rho+\alpha)$};
		\node (17) at (-2.5,-7.5) {$(-a{\color{red}-p_A}+\rho,-b{\color{red}+p_A}+\rho)$};

		%B block bottom
		\node (18) at (-3,-9) {$(-a{\color{red}-p_A}+\rho,a{\color{red}+p_A}-f+\rho+\alpha)$};
		\node (19) at (-0.5,-9.5) {$(d_A+\rho+\alpha-\epsilon,-d_A+\rho+\alpha)$};

		{\color{teal}
		\path (1) edge node [left, pos=0.5] {\tiny $A$}  (2);
		\path (1) edge node [above, pos=0.4] {\tiny $I$}  (3); 
		\path (1) edge node [left]  {\tiny $D$} (20);
		\path (1) edge node [above]  {\tiny $H$} (21);}
		
		{\color{olive}
		\path (2) edge node [above] {\tiny $S$}  (4);
		\path (2) edge node [left, pos=0.3] {\tiny $I$}  (5);
		\path (2) edge node [above] {\tiny $H$}  (6);
		\path (2) edge node [left] {\tiny $D$}  (7);
		 
		\path (3) edge node [above, pos=0.5] {\tiny $I$}  (8);
		\path (3) edge node [left] {\tiny $S$} (24); 
		\path (3) edge node [left] {\tiny $H$}  (9);
		\path (3) edge node [above] {\tiny $D$}  (10); 
		
		\path (20) edge node [below] {\tiny $I$} (23); 
		\path (20) edge node [below] {\tiny $P$} (22);}
		
		{\color{teal}
		\path (7) edge node [below] {\tiny $P$}  (11); 
		\path (7) edge node [below] {\tiny $I$}  (12);
		
		\path (10) edge node [above, pos=0.7] {\tiny $P$}  (13);
		\path (10) edge node [below] {\tiny $I$}  (14);
		
		\path (5) edge node [left] {\tiny $D$}  (15);
		\path (5) edge node [above] {\tiny $H$}  (16); 
		\path (5) edge node [above] {\tiny $I$}  (17);}
		
		{\color{olive}
		\path (15) edge node [below] {\tiny $P$}  (18);
		\path (15) edge node [below] {\tiny $I$}  (19);}
	\end{tikzpicture}
	\caption{Subgame $S_{3}$ with  Update $(a,b)\mapsto (a+p_A,b-p_A)$.}
	\label{tbl:S3}
\end{figure}

\begin{figure}
	\centering
	\begin{tikzpicture}[->,>=stealth',auto,node distance=2cm, el/.style = {inner sep=2pt, align=left, sloped}]
		\node (1) at (1.75,0.75) {\color{teal}$A$};
		
		%A block top
		\node (20) at (1,-2.25) {\color{olive} $B$};
		\node (2) at (1.75,-3.25) {\color{olive}$B$} ; 
		\node (3) at (-1.,-0.25) {\color{olive}$B$};
		\node (21) at (-1,0.5) {$(\alpha-\epsilon,\alpha)$};
		
		%B block left
		\node (22) at (-2.,-3.25) {$(-a,a-f+\alpha)$};
		\node (23) at (-3.5,-2.75) {$(d_A+\alpha-\epsilon,-d_A+\alpha)$};
				
		%B block middle
		\node (8) at (-2.5,-2) {$(-a,-b)$};
		\node (24) at (-0.,-1.25) {$(\alpha,\alpha)$};
		\node (9) at (-1.,-2.) {$(\alpha,\alpha-\epsilon)$};
		\node (10) at (-2.25,-0.5) {\color{teal}$A$};
		
		%B block right
		\node (4) at (-2.5,-4) {$({\color{red}p_B}+\rho+\alpha,{\color{red}-p_B}+\rho+\alpha)$};
		\node (5) at (1.75,-6.75) {\color{teal}$A$};
		\node (6) at (-1,-4.5) {$(\rho+\alpha,\rho+\alpha-\epsilon)$};
		\node (7) at (1,-5.) {\color{teal}$A$};

		%A block middle
		\node (11) at (-0.75,-6.25) {$(b{\color{red}+p_B}-f+\rho+\alpha,-b{\color{red}-p_B}+\rho)$};
		\node (12) at (-2.75,-5.75) {$(-d_B+\rho+\alpha,d_B+\rho+\alpha-\epsilon)$};
		
		%A block left
		\node (13) at (-5,-0.75) {$(b-f+\alpha,-b)$};
		\node (14) at (-4.25,-1.25) {$(-d_B+\alpha,d_B+\alpha-\epsilon)$};

		%A block right
		\node (15) at (1.75,-8.25) {\color{olive}$B$};
		\node (16) at (-0.5,-8) {$(\rho+\alpha-\epsilon,\rho+\alpha)$};
		\node (17) at (-2.5,-7.5) {$(-a{\color{red}+p_B}+\rho,-b{\color{red}-p_B}+\rho)$};

		%B block bottom
		\node (18) at (-3,-9) {$(-a{\color{red}+p_B}+\rho,a{\color{red}-p_B}-f+\rho+\alpha)$};
		\node (19) at (-0.5,-9.5) {$(d_A+\rho+\alpha-\epsilon,-d_A+\rho+\alpha)$};

		{\color{teal}
		\path (1) edge node [left, pos=0.5] {\tiny $A$}  (2);
		\path (1) edge node [above, pos=0.4] {\tiny $I$}  (3); 
		\path (1) edge node [left]  {\tiny $D$} (20);
		\path (1) edge node [above]  {\tiny $H$} (21);}
		
		{\color{olive}
		\path (2) edge node [above] {\tiny $S$}  (4);
		\path (2) edge node [left, pos=0.3] {\tiny $I$}  (5);
		\path (2) edge node [above] {\tiny $H$}  (6);
		\path (2) edge node [left] {\tiny $D$}  (7);
		 
		\path (3) edge node [above, pos=0.5] {\tiny $I$}  (8);
		\path (3) edge node [left] {\tiny $S$} (24); 
		\path (3) edge node [left] {\tiny $H$}  (9);
		\path (3) edge node [above] {\tiny $D$}  (10); 
		
		\path (20) edge node [below] {\tiny $I$} (23); 
		\path (20) edge node [below] {\tiny $P$} (22);}
		
		{\color{teal}
		\path (7) edge node [below] {\tiny $P$}  (11); 
		\path (7) edge node [below] {\tiny $I$}  (12);
		
		\path (10) edge node [above, pos=0.7] {\tiny $P$}  (13);
		\path (10) edge node [below] {\tiny $I$}  (14);
		
		\path (5) edge node [left] {\tiny $D$}  (15);
		\path (5) edge node [above] {\tiny $H$}  (16); 
		\path (5) edge node [above] {\tiny $I$}  (17);}
		
		{\color{olive}
		\path (15) edge node [below] {\tiny $P$}  (18);
		\path (15) edge node [below] {\tiny $I$}  (19);}
	\end{tikzpicture}
	\caption{Subgame $S_{4}$ with Update $(a,b)\mapsto (a-p_B,b+p_B)$.}
	\label{tbl:S4}
\end{figure}

Finally, the subgames $S'_3$ and $S'_4$ in \Cref{tbl:S3p,tbl:S4p} handle the same situations as $S_3$ and $S_4$, except the by $A$ partially signed closing attempt is unfair and increases $A$'s outcome by $c>0$.

\begin{figure}
	\centering
	\begin{tikzpicture}[->,>=stealth',auto,node distance=2cm, el/.style = {inner sep=2pt, align=left, sloped}]
		\node (1) at (1.75,0.75) {\color{teal}$A$};
		
		%A block top
		\node (20) at (1,-2.25) {\color{olive} $B$};
		\node (2) at (1.75,-3.25) {\color{olive}$B$} ; 
		\node (3) at (-1.,-0.25) {\color{olive}$B$};
		\node (21) at (-1,0.5) {$(\alpha-\epsilon,\alpha)$};
		
		%B block left
		\node (22) at (-2.,-3.25) {$(-a,a-f+\alpha)$};
		\node (23) at (-3.5,-2.75) {$(d_A+\alpha-\epsilon,-d_A+\alpha)$};
				
		%B block middle
		\node (8) at (-3.25,-2) {$(-a,-b)$};
		\node (24) at (-0.15,-1.25) {$({\color{red}c}+\alpha,{\color{red}-c}+\alpha)$};
		\node (9) at (-1.75,-2.) {$(\alpha,\alpha-\epsilon)$};
		\node (10) at (-2.25,-0.5) {\color{teal}$A$};
		
		%B block right
		\node (4) at (-3,-4) {$({\color{red}c-p_A}+\rho+\alpha,{\color{red}-c+p_A}+\rho+\alpha)$};
		\node (5) at (1.75,-6.75) {\color{teal}$A$};
		\node (6) at (-1,-4.5) {$(\rho+\alpha,\rho+\alpha-\epsilon)$};
		\node (7) at (1,-5.) {\color{teal}$A$};

		%A block middle
		\node (11) at (-0.75,-6.25) {$(b{\color{red}-p_A}-f+\rho+\alpha,-b{\color{red}+p_A}+\rho)$};
		\node (12) at (-2.75,-5.75) {$(-d_B+\rho+\alpha,d_B+\rho+\alpha-\epsilon)$};
		
		%A block left
		\node (13) at (-5,-0.75) {$(b-f+\alpha,-b)$};
		\node (14) at (-4.35,-1.25) {$(-d_B+\alpha,d_B+\alpha-\epsilon)$};

		%A block right
		\node (15) at (1.75,-8.25) {\color{olive}$B$};
		\node (16) at (-0.5,-8) {$(\rho+\alpha-\epsilon,\rho+\alpha)$};
		\node (17) at (-2.5,-7.5) {$(-a{\color{red}-p_A}+\rho,-b{\color{red}+p_A}+\rho)$};

		%B block bottom
		\node (18) at (-3,-9) {$(-a{\color{red}-p_A}+\rho,a{\color{red}+p_A}-f+\rho+\alpha)$};
		\node (19) at (-0.5,-9.5) {$(d_A+\rho+\alpha-\epsilon,-d_A+\rho+\alpha)$};

		{\color{teal}
		\path (1) edge node [left, pos=0.5] {\tiny $A$}  (2);
		\path (1) edge node [above, pos=0.4] {\tiny $I$}  (3); 
		\path (1) edge node [left]  {\tiny $D$} (20);
		\path (1) edge node [above]  {\tiny $H$} (21);}
		
		{\color{olive}
		\path (2) edge node [above] {\tiny $S$}  (4);
		\path (2) edge node [left, pos=0.3] {\tiny $I$}  (5);
		\path (2) edge node [above] {\tiny $H$}  (6);
		\path (2) edge node [left] {\tiny $D$}  (7);
		 
		\path (3) edge node [above, pos=0.5] {\tiny $I$}  (8);
		\path (3) edge node [left] {\tiny $S$} (24); 
		\path (3) edge node [left] {\tiny $H$}  (9);
		\path (3) edge node [above] {\tiny $D$}  (10); 
		
		\path (20) edge node [below] {\tiny $I$} (23); 
		\path (20) edge node [below] {\tiny $P$} (22);}
		
		{\color{teal}
		\path (7) edge node [below] {\tiny $P$}  (11); 
		\path (7) edge node [below] {\tiny $I$}  (12);
		
		\path (10) edge node [above, pos=0.7] {\tiny $P$}  (13);
		\path (10) edge node [below] {\tiny $I$}  (14);
		
		\path (5) edge node [left] {\tiny $D$}  (15);
		\path (5) edge node [above] {\tiny $H$}  (16); 
		\path (5) edge node [above] {\tiny $I$}  (17);}
		
		{\color{olive}
		\path (15) edge node [below] {\tiny $P$}  (18);
		\path (15) edge node [below] {\tiny $I$}  (19);}
	\end{tikzpicture}
	\caption{Subgame $S'_{3}$ with Update $(a,b)\mapsto (a+p_A,b-p_A)$.}
	\label{tbl:S3p}
\end{figure}

\begin{figure}
	\centering
	\begin{tikzpicture}[->,>=stealth',auto,node distance=2cm, el/.style = {inner sep=2pt, align=left, sloped}]
		\node (1) at (1.75,0.75) {\color{teal}$A$};
		
		%A block top
		\node (20) at (1,-2.25) {\color{olive} $B$};
		\node (2) at (1.75,-3.25) {\color{olive}$B$} ; 
		\node (3) at (-1.,-0.25) {\color{olive}$B$};
		\node (21) at (-1,0.5) {$(\alpha-\epsilon,\alpha)$};
		
		%B block left
		\node (22) at (-2.,-3.25) {$(-a,a-f+\alpha)$};
		\node (23) at (-3.5,-2.75) {$(d_A+\alpha-\epsilon,-d_A+\alpha)$};
				
		%B block middle
		\node (8) at (-3.25,-2) {$(-a,-b)$};
		\node (24) at (-0.15,-1.25) {$({\color{red}c}+\alpha,{\color{red}-c}+\alpha)$};
		\node (9) at (-1.75,-2.) {$(\alpha,\alpha-\epsilon)$};
		\node (10) at (-2.25,-0.5) {\color{teal}$A$};
		
		%B block right
		\node (4) at (-3,-4) {$({\color{red}c+p_B}+\rho+\alpha,{\color{red}-c-p_B}+\rho+\alpha)$};
		\node (5) at (1.75,-6.75) {\color{teal}$A$};
		\node (6) at (-1,-4.5) {$(\rho+\alpha,\rho+\alpha-\epsilon)$};
		\node (7) at (1,-5.) {\color{teal}$A$};

		%A block middle
		\node (11) at (-0.75,-6.25) {$(b{\color{red}+p_B}-f+\rho+\alpha,-b{\color{red}-p_B}+\rho)$};
		\node (12) at (-2.75,-5.75) {$(-d_B+\rho+\alpha,d_B+\rho+\alpha-\epsilon)$};
		
		%A block left
		\node (13) at (-5,-0.75) {$(b-f+\alpha,-b)$};
		\node (14) at (-4.35,-1.25) {$(-d_B+\alpha,d_B+\alpha-\epsilon)$};

		%A block right
		\node (15) at (1.75,-8.25) {\color{olive}$B$};
		\node (16) at (-0.5,-8) {$(\rho+\alpha-\epsilon,\rho+\alpha)$};
		\node (17) at (-2.5,-7.5) {$(-a{\color{red}+p_B}+\rho,-b{\color{red}-p_B}+\rho)$};

		%B block bottom
		\node (18) at (-3,-9) {$(-a{\color{red}+p_B}+\rho,a{\color{red}-p_B}-f+\rho+\alpha)$};
		\node (19) at (-0.5,-9.5) {$(d_A+\rho+\alpha-\epsilon,-d_A+\rho+\alpha)$};

		{\color{teal}
		\path (1) edge node [left, pos=0.5] {\tiny $A$}  (2);
		\path (1) edge node [above, pos=0.4] {\tiny $I$}  (3); 
		\path (1) edge node [left]  {\tiny $D$} (20);
		\path (1) edge node [above]  {\tiny $H$} (21);}
		
		{\color{olive}
		\path (2) edge node [above] {\tiny $S$}  (4);
		\path (2) edge node [left, pos=0.3] {\tiny $I$}  (5);
		\path (2) edge node [above] {\tiny $H$}  (6);
		\path (2) edge node [left] {\tiny $D$}  (7);
		 
		\path (3) edge node [above, pos=0.5] {\tiny $I$}  (8);
		\path (3) edge node [left] {\tiny $S$} (24); 
		\path (3) edge node [left] {\tiny $H$}  (9);
		\path (3) edge node [above] {\tiny $D$}  (10); 
		
		\path (20) edge node [below] {\tiny $I$} (23); 
		\path (20) edge node [below] {\tiny $P$} (22);}
		
		{\color{teal}
		\path (7) edge node [below] {\tiny $P$}  (11); 
		\path (7) edge node [below] {\tiny $I$}  (12);
		
		\path (10) edge node [above, pos=0.7] {\tiny $P$}  (13);
		\path (10) edge node [below] {\tiny $I$}  (14);
		
		\path (5) edge node [left] {\tiny $D$}  (15);
		\path (5) edge node [above] {\tiny $H$}  (16); 
		\path (5) edge node [above] {\tiny $I$}  (17);}
		
		{\color{olive}
		\path (15) edge node [below] {\tiny $P$}  (18);
		\path (15) edge node [below] {\tiny $I$}  (19);}
	\end{tikzpicture}
	\caption{Subgame $S'_{4}$ with Update $(a,b)\mapsto (a-p_B,b+p_B)$.}
	\label{tbl:S4p}
\end{figure}
